# Supplementary material for: Spatial Relation Graph and Graph Convolutional Network for Object Goal Navigation
Source: arXiv:2208.13031 source file (2022-08-27)
Supplement: Supplementary file 1 [file supplimentary_material.tex]

\cleardoublepage

\begin{table*}[t]
\caption{19 target objects - 6 scenes -spatial relational graph .}
\centering
\begin{tabular}{p{0.1\linewidth}p{0.1\linewidth}p{0.1\linewidth}p{0.1\linewidth}p{0.1\linewidth}p{0.1\linewidth}p{0.1\linewidth}p{0.1\linewidth}}
\hline
Scene & 17DRP5sb8fy & rPc6DW4iMge & S9hNv5qa7GM & b8cTxDM8gDG & EDJbREhghzL & 2azQ1b91cZZ & Average\\
\hline
Success & 97.2\% & 93.2\% & 90.4\% & 95.199\% & 96.8\% & 92.0\% & 94.133\%\\
SPL & 0.71217 & 0.63095203 & 0.62110938 & 0.725328 & 0.68575 & 0.5738964 & 0.658\%\\
SoftSPL & 0.72713 & 0.644370 & 0.6442022 & 0.74555085 & 0.71081 & 0.6039638 & 0.67931\\
DTS & 0.01170 & 0.45190313 & 0.6674027 & 0.29111623 & 0.05681 & 0.3497 & 0.3047\\
\hline
\end{tabular}
\end{table*}

\begin{table*}[t]
\caption{target object- BED - 6 scenes - random object .}
\centering
\begin{tabular}{p{0.1\linewidth}p{0.1\linewidth}p{0.1\linewidth}p{0.1\linewidth}p{0.1\linewidth}p{0.1\linewidth}p{0.1\linewidth}p{0.1\linewidth}}
\hline
Scene & 17DRP5sb8fy & rPc6DW4iMge & S9hNv5qa7GM & b8cTxDM8gDG & EDJbREhghzL & 2azQ1b91cZZ & Average\\
\hline
Success & 98.0-98.0\% & 82.0-82.0\% & 22.0-22.0\% & 28.0-28.0000\% & 40.0-40.0\% & 90.0-90.0\% & 60\%\\
SPL & 0.7874150 & 0.3127048 & 0.11991 & 0.2192129 & 0.12750 & 0.52414652 & 0.3484\\

\hline
\end{tabular}
\end{table*}

\begin{table*}[t]
\caption{target object- BED - 6 scenes - spatial relation graph.}
\centering
\begin{tabular}{p{0.1\linewidth}p{0.1\linewidth}p{0.1\linewidth}p{0.1\linewidth}p{0.1\linewidth}p{0.1\linewidth}p{0.1\linewidth}p{0.1\linewidth}}
\hline
Scene & 17DRP5sb8fy & rPc6DW4iMge & S9hNv5qa7GM & b8cTxDM8gDG & EDJbREhghzL & 2azQ1b91cZZ & Average\\
\hline
Success & 100.0-100.0\% & 99.0-99.0\% & 100.0-100.0\% & 100-100\% & 100-100\% & 100-100\% & 99.83\\
SPL & 0.8838 & 0.5607001 & 0.60738379  & 0.803218 & 0.529856627 & 0.6842170 & 0.67803\\

\hline
\end{tabular}
\end{table*}

\begin{table*}[t]
\caption{target object- TOWEL - 6 scenes - random object .}
\centering
\begin{tabular}{p{0.1\linewidth}p{0.1\linewidth}p{0.1\linewidth}p{0.1\linewidth}p{0.1\linewidth}p{0.1\linewidth}p{0.1\linewidth}p{0.1\linewidth}}
\hline
Scene & 17DRP5sb8fy & rPc6DW4iMge & S9hNv5qa7GM & b8cTxDM8gDG & EDJbREhghzL & 2azQ1b91cZZ & Average\\
\hline
Success & 99.0-99.0\% & 2.0-2.0\% & 61.0-61.0\% & 41.0-41.0\% & 57.0-56.999\% & 2.0-2.0\% & 43.66\%\\
SPL & 0.544416 & 0.014903 & 0.2072007 & 0.21482 & 0.26191 & 0.0034244455 & 0.2075\\

\hline
\end{tabular}
\end{table*}

\begin{table*}[t]
\caption{target object- TOWEL - 6 scenes - spatial relational graph .}
\centering
\begin{tabular}{p{0.1\linewidth}p{0.1\linewidth}p{0.1\linewidth}p{0.1\linewidth}p{0.1\linewidth}p{0.1\linewidth}p{0.1\linewidth}p{0.1\linewidth}}
\hline
Scene & 17DRP5sb8fy & rPc6DW4iMge & S9hNv5qa7GM & b8cTxDM8gDG & EDJbREhghzL & 2azQ1b91cZZ & 86.66\%\\
\hline
Success & 100.0-100.0\% & 58.0-57.99\% & 96.0-96.0\% & 95.0-95.0\% & 88.0-88.0\% & 83.0-83.0\% & 86.66\%\\
SPL & 0.7289 & 0.4545 & 0.52725  & 0.359044 & 0.60414 & 0.48103 & 0.5258\\

\hline
\end{tabular}
\end{table*}

\begin{table*}[t]
\caption{target object- CHAIR - 6 scenes - random object .}
\centering
\begin{tabular}{p{0.1\linewidth}p{0.1\linewidth}p{0.1\linewidth}p{0.1\linewidth}p{0.1\linewidth}p{0.1\linewidth}p{0.1\linewidth}p{0.1\linewidth}}
\hline
Scene & 17DRP5sb8fy & rPc6DW4iMge & S9hNv5qa7GM & b8cTxDM8gDG & EDJbREhghzL & 2azQ1b91cZZ & Average\\
\hline
Success & 98.0-98.0\% & 97.0-97.0\% & 55.0-55.000\% & 92.0-92.0\% & 97.0-97.0\% & 89.0-89.0\% & 88\%\\
SPL & 0.7487202383503 & 0.630283 & 0.20917 & 0.727183 & 0.88803 & 0.4916503 & 0.615\\

\hline
\end{tabular}
\end{table*}

\begin{table*}[t]
\caption{target object- CHAIR - 6 scenes - spatial relational graph .}
\centering
\begin{tabular}{p{0.1\linewidth}p{0.1\linewidth}p{0.1\linewidth}p{0.1\linewidth}p{0.1\linewidth}p{0.1\linewidth}p{0.1\linewidth}p{0.1\linewidth}}
\hline
Scene & 17DRP5sb8fy & rPc6DW4iMge & S9hNv5qa7GM & b8cTxDM8gDG & EDJbREhghzL & 2azQ1b91cZZ & Average\\
\hline
Success & 99.0-99.0\% & 100.0-100.0\% & 73.0-73.0\% & 100-100\% & 97-97\% & 94-94\% & 93.83\%\\
SPL & 0.803899 & 0.684538 & 0.499564343  & 0.860181 & 0.8696 & 0.462590 & 0.696\\

\hline
\end{tabular}
\end{table*}

\begin{table*}[t]
\caption{target object- SHOWER - 6 scenes - random object .}
\centering
\begin{tabular}{p{0.1\linewidth}p{0.1\linewidth}p{0.1\linewidth}p{0.1\linewidth}p{0.1\linewidth}p{0.1\linewidth}p{0.1\linewidth}p{0.1\linewidth}}
\hline
Scene & 17DRP5sb8fy & rPc6DW4iMge & S9hNv5qa7GM & b8cTxDM8gDG & EDJbREhghzL & 2azQ1b91cZZ & Average\\
\hline
Success & 73.0-73.0\% & 79.0-79.0\% & 44.0-44.0\% & 58.0-57.999\% & 62.0-62.0\% & 62.0-62.0\% & 63\%\\
SPL & 0.24856 & 0.262345 & 0.18526717 & 0.46956 & 0.3318 & 0.15955 & 0.2761\\

\hline
\end{tabular}
\end{table*}

\begin{table*}[t]
\caption{target object- SHOWER - 6 scenes - spatial relational graph .}
\centering
\begin{tabular}{p{0.1\linewidth}p{0.1\linewidth}p{0.1\linewidth}p{0.1\linewidth}p{0.1\linewidth}p{0.1\linewidth}p{0.1\linewidth}p{0.1\linewidth}}
\hline
Scene & 17DRP5sb8fy & rPc6DW4iMge & S9hNv5qa7GM & b8cTxDM8gDG & EDJbREhghzL & 2azQ1b91cZZ & Average\\
\hline
Success & 93.0-93.0\% & 81.0-81.0\% & 68.0-68.0\% & 93.0-93.0\% & 90.0-90.0\% & 100.0-100.0\% & 87.5\%\\
SPL & 0.564670147 & 0.3739251 & 0.34659  & 0.684873 & 0.55484 & 0.603816768 & 0.521\\

\hline
\end{tabular}
\end{table*}

\begin{table*}[t]
\caption{target object- PICTURE - 6 scenes - random object .}
\centering
\begin{tabular}{p{0.1\linewidth}p{0.1\linewidth}p{0.1\linewidth}p{0.1\linewidth}p{0.1\linewidth}p{0.1\linewidth}p{0.1\linewidth}p{0.1\linewidth}}
\hline
Scene & 17DRP5sb8fy & rPc6DW4iMge & S9hNv5qa7GM & b8cTxDM8gDG & EDJbREhghzL & 2azQ1b91cZZ & Average\\
\hline
Success & 37.0-37.0\% & 45.0-45.0\% & 17.0-17.0\% & 71.0-71.0\% & 58.0-57.999\% & 9.0-9.0\% & 39.5\%\\
SPL & 0.3671 & 0.40025 & 0.1290 & 0.6759 & 0.51302 & 0.060869 & 0.3576\\

\hline
\end{tabular}
\end{table*}

\begin{table*}[t]
\caption{target object- PICTURE - 6 scenes - spatial relational graph .}
\centering
\begin{tabular}{p{0.1\linewidth}p{0.1\linewidth}p{0.1\linewidth}p{0.1\linewidth}p{0.1\linewidth}p{0.1\linewidth}p{0.1\linewidth}p{0.1\linewidth}}
\hline
Scene & 17DRP5sb8fy & rPc6DW4iMge & S9hNv5qa7GM & b8cTxDM8gDG & EDJbREhghzL & 2azQ1b91cZZ & Average\\
\hline
Success & 100.0-100.0\% & 99.0-99.0\% & 86.0-86.0\% & 95.0-95.0\% & 100-100\% & 90-90\% & 95\%\\
SPL & 0.9585802 & 0.7968499 & 0.64060811  & 0.77609 & 0.75929 & 0.4618838 & 0.7321\\

\hline
\end{tabular}
\end{table*}
